# Supplementary material for: Upper bounds of spin-density wave energies in the homogeneous electron gas
Source: arXiv:1507.06884 source file (2015-07-24)
Supplement: Supplementary file 1 [file Supp-Energies.pdf]

# Energies and potential of the Fermi gas of the truncated sphere $\mathcal{F}$

F. Delyon,[1,2] B. Bernu,[2] L. Baguet,[2] and M. Holzmann[2,3]

[1]*CPHT, UMR 7644 of CNRS, École Polytechnique, F-91128 Palaiseau Cedex, France*
[2]*LPTMC, UMR 7600 of CNRS, UPMC, Paris-Sorbonne, F-75252 Paris Cedex 05, France*
[3]*LPMMC, UMR 5493 of CNRS, Université J. Fourier, BP 166, F-38042 Grenoble Cedex, France*

Here we provide some details on the technical derivation of the energies, Eq. (4) of the letter, and potentials, Eq. 7-8 of the letter.

## I. ENERGY

We recall here the first equations of the letter. The Fermi gas energy per particle in Hartree units is

$$E_{\mathrm{FG}}^{\mathcal{F}} = \frac{a_K R^5}{r_s^2} K_{\mathrm{FG}} - \frac{a_V R^4}{r_s} V_{\mathrm{FG}} \quad (1)$$

$$K_{\mathrm{FG}} = \int_{\mathcal{F}_\uparrow + \mathcal{F}_\downarrow} d\mathbf{k}\, k^2 \quad (2)$$

$$V_{\mathrm{FG}} = \int_{\mathcal{F}_\uparrow \times \mathcal{F}_\uparrow + \mathcal{F}_\downarrow \times \mathcal{F}_\downarrow} d\mathbf{k}\, d\mathbf{k}'\, \frac{1}{|k-k'|^2} \quad (3)$$

where $\mathcal{F}_\uparrow$ and $\mathcal{F}_\downarrow$ are defined in the Fig. 1 of the letter, and $a_V = \frac{3}{32\pi^3}\left(\frac{9\pi}{4}\right)^{1/3}$, $a_K/a_V = 2\pi^2\left(\frac{9\pi}{4}\right)^{1/3} \approx 37.9$ and $\mathbf{k}$ is in $k_F$ units. Keeping the total volume of $\mathcal{F}$ constant leads to the relation between the radius $R$ of the sphere, $\epsilon$ and $h$ (see Fig. 1 of the letter)

$$R^3 = \frac{4}{4 - 3\epsilon^2(1-2h) + \epsilon^3(1-3h)} \quad (4)$$

In the following we use $c = 1-\epsilon$ (the largest $k_z$ of the truncated sphere) and $r = \sqrt{1-c^2} = \sqrt{\epsilon(2-\epsilon)}$.

### A. Kinetic energy

Eq. (2) reads

$$K_{\mathrm{FG}} = 2\int_{\mathcal{F}_\uparrow} d\mathbf{k}\, \mathbf{k}^2 \quad (5)$$

$$= 2\int_{-1}^{1-\epsilon} dk_z \int_0^{\sqrt{1-k_z^2}} d\rho\, 2\pi\rho\,(k_z^2+\rho^2) + 2\int_{1-\epsilon}^{1-\epsilon+h\epsilon} dk_z \int_0^r d\rho\, 2\pi\rho\,(k_z^2+\rho^2) \quad (6)$$

One finds

$$K_{\mathrm{FG}} = 2\times\frac{4\pi}{5} \times\Big(1 - \frac{5\epsilon^2}{4}(1-2h) + \frac{5\epsilon^3}{4}(1-2h)(1-h) + \frac{5\epsilon^4}{24}(4h^3-18h^2+12h-3) - \frac{\epsilon^5}{24}(10h^3-30h^2+15h-3)\Big) \quad (7)$$

Thus the increase of kinetic energy reads

$$\Delta K_{\mathrm{FG}} = \frac{a_K}{r_s^2}\left(R^5 K_{\mathrm{FG}} - 2\times\frac{4\pi}{5}\right) \approx \frac{a_K\pi}{r_s^2}\left[\left((2h-1)^2+\frac{1}{3}\right)\epsilon^3 + \left(\frac{4}{3}(h-2)^3 - 10h + \frac{55}{6}\right)\epsilon^4 + ...\right] \quad (8)$$

### B. Potential Energy

From Eq. (3), we have

$$V_{\mathrm{FG}} = 2\int_{\mathbf{k},\mathbf{k}'\in\mathcal{F}_\uparrow} d\mathbf{k}\, d\mathbf{k}'\, \frac{1}{\|\mathbf{k}^2 - \mathbf{k}'^2\|} \quad (9)$$

As $\mathcal{F}_\uparrow$ is the sum of two volumes: the truncated sphere $\mathcal{T}$ and the cylinder $\mathcal{C}$, $V_{\mathrm{FG}}$ is decomposed on integrals on $\mathcal{T}\times\mathcal{T}$, $\mathcal{C}\times\mathcal{C}$ and $\mathcal{T}\times\mathcal{C}$:

$$V_{\mathrm{FG}} = 2V_{\mathcal{T}} + 4V_{\mathcal{T}\mathcal{C}} + 2V_{\mathcal{C}} \quad (10)$$

Integrating $\mathbf{k}$ on a disk of radius $r_1$ and $\mathbf{k}'$ on a disk of radius $r_2$ gives, with $A = k_z - k_z'$ (we have divided by $\pi^2$ to simplify the formula):

$$I(A,r_1,r_2) = \int_0^{r_1} d\rho\,\rho \int_0^{r_2} d\rho'\rho' \int_0^{2\pi} \frac{2\pi}{A^2+\rho^2+\rho'^2-2\rho\rho'\cos\theta}\frac{d\theta}{\pi^2}$$
$$= (r_1^2 - r_2^2)\ln(A^2 - r_1^2 + r_2^2 + Y) + r_2^2\ln(A^2+r_1^2+r_2^2+Y) - r_1^2\ln(2A^2) - \frac{1}{2}\left(A^2+r_2^2+r_1^2-Y\right)$$

$$Y = \sqrt{(A^2+(r_1-r_2)^2)(A^2+(r_1+r_2)^2)} \quad (11)$$

$$= \sqrt{(A^2+r_1^2+r_2^2)^2 - 4r_1^2r_2^2}. \quad (12)$$

#### 1. Self potential energy $V_{\mathcal{T}}$

We have

$$V_{\mathcal{T}} = \int_{\mathbf{k},\mathbf{k}'\in\mathcal{T}} d\mathbf{k}\, d\mathbf{k}'\, \frac{1}{\|\mathbf{k}-\mathbf{k}'\|^2} \quad (13)$$

$$= \pi^2 \int_{-1}^{c} dk_z \int_{-1}^{c} dk_z' J(k_z,k_z') \quad (14)$$

$$J(k_z,k_z') = I(k_z-k_z', \sqrt{1-k_z^2}, \sqrt{1-k_z'^2}) \quad (15)$$

Because $J(k_z,k'_z)=J(k'_z,k_z)$, we get

$$V_{\mathcal{T}} =2\pi^2\int_{-1}^{c} dk_z \int_{-1}^{k_z} dk'_z J(k_z,k'_z) \tag{16}$$

For $-1<k'_z<k_z<c$, $J(k_z,k'_z)$ simplifies into

$$\begin{aligned} J(k_z,k'_z) = &\left({k'_z}^2+{k_z}^2-2\right)\ln\left(k_z-k'_z\right)\\ &+\left(1-{k'_z}^2\right)\ln\left(1-k'_z\right)\\ &+\left(1-{k_z}^2\right)\ln\left(k_z+1\right)\\ &+k_z\,k'_z-k'_z+k_z-1 \end{aligned}\tag{17}$$

Integrating over $k_z$ and $k'_z$ gives

$$\begin{aligned} V_{\mathcal{T}} =&\frac{\pi^2}{6}\big[(c+3)(1-c)^3\ln(1-c)\\ &-(3-c)(1+c)^3\ln(1+c)\\ &+(1+c)(9+5c+c^2-3c^3)+16c\ln 2\big] \end{aligned}\tag{18}$$

If $\epsilon=0$, then $c=1$ and we get $R=1$ and $R^4V_{\mathcal{T}}=4\pi^2$. At small $\epsilon$ we find

$$\begin{aligned} R^4V_{\mathcal{T}}-4\pi^2\approx &-8\pi^2h\epsilon^2+\pi^2\left(\frac{7}{9}-\frac{2t}{3}+4h\right)\epsilon^3\\ &+\pi^2\left(-\frac{53}{72}+\frac{t}{6}+14h^2-6h\right)\epsilon^4+... \end{aligned}\tag{19}$$

where $t=\ln(2/\epsilon)$.

### 2. Self potential energy $V_{\mathcal{C}}$

$V_{\mathcal{C}}$ is defined as

$$\begin{aligned} V_{\mathcal{C}} = &\int_{\mathbf{k},\mathbf{k}'\in\mathcal{C}} d\mathbf{k}\,d\mathbf{k}'\,\frac{1}{\|\mathbf{k}-\mathbf{k}'\|^2} &(20)\\ =&\pi^2\int_0^{\epsilon h} dk_z\int_0^{\epsilon h} dk'_z I(k_z-k'_z,r,r) &(21)\\ I(k_z-k'_z,r,r) =& r^2 I\left(\frac{k_z-k'_z}{r},1,1\right) &(22) \end{aligned}$$

where $I(A,1,1)=-\ln A^2-\left(A^2+2-\sqrt{A^2+4}\,|A|\right)/2+2\,\mathrm{arcsinh}\,(|A|/2)$ is an even function of $A$. Using $\epsilon h=\mu r$,

$$\begin{aligned} V_{\mathcal{C}} =&\frac{\pi^2r^4}{12}\left(\mu((\mu^2-26)\sqrt{\mu^2+4}+64)+\mu^2(24-\mu^2)\right.\\ &\left.-24\left[(1-\mu^2)\,\mathrm{arcsinh}\,\frac{\mu}{2}+\mu^2\ln\mu\right]\right). \end{aligned}\tag{23}$$

At small $\epsilon$, we get

$$\begin{aligned} \frac{R^4V_{\mathcal{C}}}{\pi^2} \approx&2h^2(t-2u+2)\epsilon^3+\frac{2\sqrt{2}}{3}h^3\epsilon^{7/2}\\ &+h^2\left(2u-t-\frac{h^2}{12}-3\right)\epsilon^4+... \end{aligned}\tag{24}$$

where $t=\ln(2/\epsilon)$ and $u=\ln h$.

### 3. Potential energy $V_{\mathcal{TC}}$

It is defined as

$$\begin{aligned} V_{\mathcal{TC}} =& \int_{\mathbf{k}\in\mathcal{C},\,\mathbf{k}'\in\mathcal{T}} d\mathbf{k}\,d\mathbf{k}'\,\frac{1}{\|\mathbf{k}-\mathbf{k}'\|^2} &(25)\\ =&\pi^2\int_c^{c+\epsilon h} dk_z\int_{-1}^{c} dk'_z\,I(k_z-k'_z,r,\sqrt{1-k'_z}) &(26) \end{aligned}$$

In Eq.12, all terms in log depends on $A^2+r_2^2$ which is linear in $k'_z$ ($r_2=\sqrt{1-k'^2_z}$). Then setting $k_z=c+z$ ($z\in[0,\epsilon h]$) and $k'_z=c-x$, ($x\in[0,1+c]$)

$$\begin{aligned} J(x,z) =&I(z+x,r,\sqrt{1-k'^2_z}) &(27)\\ =&x(x-2c)\ln(2cx+2xz+z^2+Y)\\ &-(x^2-2cx-r^2)\ln(2cx+2r^2+2xz+z^2+Y)\\ &-r^2\ln(2(z+x)^2)\\ &+\frac{(c-x)^2-(z+x)^2-1-r^2+Y}{2}\\ Y^2 =&\frac{(2S^2x+z(z^2+cz+2r^2))^2+z^2r^2(2c+z)^2}{S^2} &(28)\\ S =&\sqrt{(z+c)^2+r^2} &(29) \end{aligned}$$

Then

$$\begin{aligned} V_{\mathcal{TC}} =&\pi^2\int_0^{\epsilon h} dz\,V(z) &(30)\\ V(z) =&\int_0^{1+c} dx\,J(x,z) &(31)\\ =&\frac{1}{3}\Big[-\left(z^3+3cz^2+2(1-3c+c^3)\right)L_1\\ &+\left(S^2-3\right)S\,L_2+2L_3\\ &+2\left(1+c+z\right)^2\left(c+z-2\right)\ln\left(1+c+z\right)\\ &-\left(z^3+3cz^2-6r^2z-2\right)\ln z\\ &+\left(z^3+3cz^2-6c+2c^3\right)\ln 2-\frac{c+2z}{2}zS_1\\ &+z^3+\frac{cz^2}{2}+r^2(2z+3c+2)\Big] &(32) \end{aligned}$$

with

$$\begin{aligned} S_1 =&\sqrt{z^2+4r^2} &(33)\\ L_1 =&\ln\left(S_1+z\right) &(34)\\ L_2 =&\ln\frac{z(S+S_1+1)(S+S_1-1)}{2(S+1)^2(S+z+c)} &(35)\\ L_3 =&\ln\left((S_1+z)(z+2+2c)+4(1+c)\right) &(36) \end{aligned}$$

The last integration is done after series expansion in $\epsilon$:

$$\begin{aligned} \frac{R^4V_{\mathcal{TC}}}{\pi^2} \approx&4h\epsilon^2\\ &+\left((1-2h)t+h(2u-1)-\frac{7}{2}\right)h\epsilon^3+O(\epsilon^4) \end{aligned}\tag{37}$$

#### 4. Potential energy $V_{\rm FG}$

The total potential energy, Eq. 10, is given by collecting the results of Eqs. 19, 24 and 37. The potential energy of the sphere is $V_{\mathcal{S}} = 4\pi^2$ (recovered here with $\epsilon = h = 0$). The variation of potential energy $V_{\rm FG} - 2V_{\mathcal{S}}$ becomes at the leading order

$$\frac{R^4 V_{\rm FG} - 2V_{\mathcal{S}}}{\pi^2} = \left[-\left((2h-1)^2+\frac{1}{3}\right)t+(2h-1)^2-2h+\frac{5}{9}\right]\epsilon^3 + O(\epsilon^{7/2}) \qquad (38)$$

#### 5. Fermi gas energy $E_{\rm FG}$

Putting together Eqs. (8) and (38) we recover Eq. (4) of the letter:

$$\Delta E^{\mathcal{F}}_{\rm FG} \approx \frac{2\pi^2 a_V \epsilon^3}{r_s}\left[\alpha(\gamma-1)-\frac{1}{9}+h\right] \qquad (39)$$

with $\alpha = 2(h-\frac{1}{2})^2+\frac{1}{6}$ and $\gamma = t+\gamma_0$, where $t = \ln\frac{2}{\epsilon}$ and $\gamma_0 = \frac{a_K}{a_V \pi r_s}$.

## II. POTENTIAL

Here we calculate the potential created by $\mathcal{F}$:

$$V_{\mathcal{F}}(\mathbf{k}) = \int_{\mathcal{F}} d\mathbf{k}' \frac{1}{\|\mathbf{k}'-\mathbf{k}\|^2} = \int_{\partial\mathcal{F}} dS' \frac{\mathbf{k}'-\mathbf{k}}{\|\mathbf{k}'-\mathbf{k}\|^2} \qquad (40)$$

where $\partial\mathcal{F}$ designs the surface of $\mathcal{F}$. We use cylindrical coordinates $\mathbf{k}' = (\mathbf{q}', k'_z)$. It is decomposed in three parts: *i)* the spherical part of the truncated sphere surface, with $\|\mathbf{k}'\| = 1$ and $k'_z < 1-\epsilon$, *ii)* the vertical side of the cylinder, with $\|\mathbf{q}'\| = r$ and $1-\epsilon < k'_z < 1-\epsilon+h\epsilon$, and *iii)* the top horizontal side of the cylinder, with $\|\mathbf{q}'\| < r$ and $k'_z = 1-\epsilon+h\epsilon$, see Fig.1 of the letter.

The contribution of the truncated sphere reads:

$$I_{\mathcal{T}} = \int_{-1}^{c} dk'_z \int_0^{2\pi} d\phi' \frac{1-k_z k'_z - qq'\cos\phi'}{k^2+k'^2-2k_z k'_z-2qq'\cos\phi'} \qquad (41)$$

$$=(1+c)\pi+\frac{1-k^2}{2}\int_{-1}^{c} dk'_z \int_0^{2\pi} \frac{d\phi'}{k^2+1-2k_z k'_z-2qq'\cos\phi'}$$

$$=(1+c)\pi+\pi(1-k^2)\int_{-1}^{c}\frac{dk'_z}{\sqrt{(k^2+1-2k_z k'_z)^2-4q^2q'^2}}$$

$$=(1+c)\pi+\pi\frac{1-k^2}{2k}\ln\frac{\Gamma-A}{(k-1)^2(k-kz)} \qquad (42)$$

$$=(1+c)\pi+\pi\frac{1-k^2}{2k}\ln\frac{(k+k_z)(k+1)^2}{\Gamma+A} \qquad (43)$$

$$A = k_z(1+k^2)-2ck^2 \qquad (44)$$

$$\Gamma^2 = A^2+q^2(k^2-1)^2 \qquad (45)$$

where $c = 1-\epsilon$.

The contribution of the vertical side of the cylinder reads, with $r = \sqrt{1-c^2} = \sqrt{\epsilon(2-\epsilon)}$, and $\bar{c} = c+h\epsilon$:

$$I_{\mathcal{C},1} = \int_c^{\bar{c}} dk'_z \int_0^{2\pi} d\phi' \frac{r-q\cos\phi'}{(k_z-k'_z)^2+r^2+q^2-2rq\cos\phi'} \qquad (46)$$

With $k_z = \bar{c}-z$ and $k'_z = \bar{c}-z'$, we have

$$I_{\mathcal{C},1} = \int_0^{h\epsilon} dz' \int_0^{2\pi} d\phi' \frac{r-q\cos\phi'}{(z-z')^2+r^2+q^2-2rq\cos\phi'} \qquad (47)$$

$$= \frac{\pi}{r}\int_0^{h\epsilon} dz'\left(1-\frac{(z-z')^2+q^2-r^2}{\sqrt{((z-z')^2+q^2+r^2)^2-4q^2r^2}}\right)$$

$$= \pi\left(\frac{h\epsilon}{r}+F(z-h\epsilon)-F(z)\right) \qquad (48)$$

$$F(z) = 2\frac{q-r}{q+r}\mathcal{E}_F(a,\, b)+\frac{(q-r)^2}{r(q+r)}\mathcal{E}_\pi(a,\, 1,\, b) \qquad (49)$$

$$a = \frac{z}{\sqrt{(q-r)^2+z^2}} \qquad b = \frac{2\sqrt{qr}}{q+r} \qquad (50)$$

where $\mathcal{E}_F(a,b)$, $\mathcal{E}_\pi(a,1,b)$ are the incomplete Elliptic integral[1] F and Pi, respectively.

The surface integral at $k'_z = \bar{c}$ reads

$$I_{\mathcal{C},2} = \int_0^r q'dq' \int_0^{2\pi} d\phi' \frac{\bar{c}-k_z}{(\bar{c}-k_z)^2+q'^2+q^2-2qq'\cos\phi'}$$

$$=\pi z\int_0^{r^2} du \frac{1}{\sqrt{(z^2+q^2+u)^2-4q^2u}} \qquad (51)$$

$$=\pi z\ln\frac{2q^2}{q^2-z^2-r^2+D} \qquad (52)$$

$$=\pi z\ln\frac{z^2-q^2+r^2+D}{2z^2} \qquad (53)$$

$$D =\sqrt{z^2+(q+r)^2}\sqrt{z^2+(q-r)^2} \qquad (54)$$

Finally the total potential is given by

$$V_{\mathcal{F}} = I_{\mathcal{T}}+I_{\mathcal{C},1}+I_{\mathcal{C},2}. \qquad (55)$$

We recover the potential of the sphere $\mathcal{S}$ for $\epsilon = 0$ ($I_{\mathcal{C},1} = I_{\mathcal{C},2} = 0$)

$$V_{\mathcal{S}} = 2\pi+\pi\frac{1-k^2}{2k}\ln\frac{(k+1)^2}{(k-1)^2} \qquad (56)$$

### A. Potential at $q = 0$

Setting $\mathbf{k} = (0, k_z)$, i.e. $k_z^2 = k^2$, we get

$$I_{\mathcal{T}} =(1+c)\pi+\pi\frac{1-k^2}{2k}\ln\frac{(k+1)^2}{2\epsilon k+(1-k)^2} \qquad (57)$$

In Eq.50, for $q = 0$, we have $b = 0$ and

$$\mathcal{E}_F(a,0) = \arcsin a = \arctan\frac{z}{r} \qquad (58)$$

$$\mathcal{E}_\pi(a,1,0) = \frac{z}{r} \qquad (59)$$

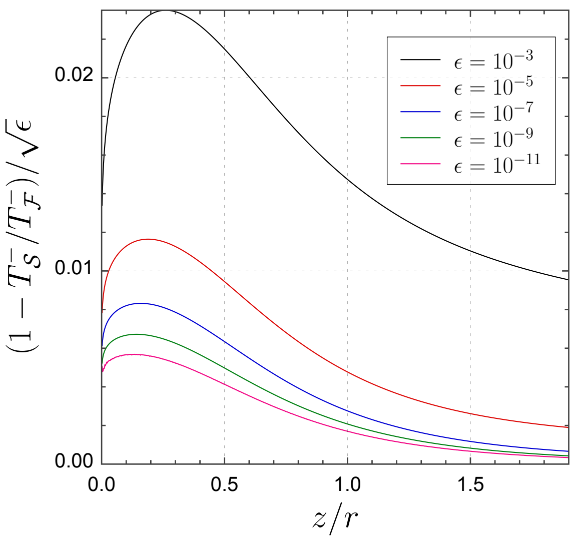


FIG. 1: Relative difference between $T^-_{\mathcal{F}}1$ and $T^-_{\mathcal{S}}1$ for various values of $\epsilon$ (Note the scaling in $\sqrt{\epsilon}$). For comparison, $T^-_{\mathcal{S}}1(z=r) \approx \pi(\ln 2 + n \ln 10)$ for $\epsilon = 10^{-n}$. Thus the relative difference is already of the order of $10^{-3}$ at $\epsilon = 10^{-3}$ and decreases roughly as $\sqrt{\epsilon}$.

Thus we get

$$I_{\mathcal{C},1} = 2\pi \left( \arctan \frac{z}{r} - \arctan \frac{z - h\epsilon}{r} \right) \tag{60}$$

and

$$I_{\mathcal{C},2} = \pi z \ln \frac{z^2 + r^2}{z^2} \tag{61}$$

For $\epsilon = 0$, then $r = 0$ and we recover the potential of the sphere.

### B. Evaluation of $T^-1$

Using the definition of Eq. (8) of the letter, we have

$$T^-_{\mathcal{F}}1 = V_{\mathcal{F}}(\mathbf{k}) - V_{\mathcal{F}}(\tilde{\mathbf{k}})$$

where $V_{\mathcal{F}}(\mathbf{k})$ is defined by Eq.56. If $\mathcal{F}$ is replace by the sphere $\mathcal{S}$ of radius 1, we obtain

$$T^-_{\mathcal{S}}1 = V_{\mathcal{S}}(1 - z) - V_{\mathcal{S}}(1 + z) \approx 4\pi z \ln \frac{2}{z} + O(z^3) \tag{62}$$

First, we compare the $T^-_{\mathcal{F}}1$ and $T^-_{\mathcal{S}}1$ along the line $q = 0$. Fig.1 shows that the relative difference $1 - T^-_{\mathcal{S}}1(z,0)/T^-_{\mathcal{F}}1(z,0)$ scales roughly as $\sqrt{\epsilon}$. Thus at small $\epsilon$, we can replace $T^-_{\mathcal{F}}1(z,0)$ by $T^-_{\mathcal{S}}1(z,0)$.

Fig.2 shows the variations $T^-_{\mathcal{F}}1(z,q)$ with $q$. These variations scale as $\epsilon$ at $z \gg \epsilon$ and as $\sqrt{\epsilon}$ in a domain of $q$ close to 1 ($1 - q \approx \epsilon$).

Fig.1 and Fig.2 show that as $\epsilon$ goes to 0, the potential created by $\mathcal{F}$ can be replaced by that of the sphere $\mathcal{S}$ to compute $T^-1$.

## III. 1-D APPROXIMATION

Scalar product with $T^\pm$ are simplified when the function is one-dimensional. We evaluate the following integral (Eq. (20) of the letter):

$$\begin{aligned}
G(x) =& \frac{1}{\pi^2 r^2} \int_{q^2, q'^2 < r^2} d\mathbf{q}\, d\mathbf{q}' \frac{1}{r^2 x^2 + (\mathbf{q} - \mathbf{q}')^2} && (63)\\
=& \frac{2}{\pi r^2} \int_0^r q\, dq \int_0^r q'\, dq' \int_0^{2\pi} dt && (64)\\
& \times \frac{1}{r^2 x^2 + q^2 + q'^2 - 2qq' \cos t} && (65)\\
=& \frac{2}{\pi} \int_0^1 q\, dq \int_0^1 q'\, dq' \int_0^{2\pi} dt && (66)\\
& \times \frac{1}{x^2 + q^2 + q'^2 - 2qq' \cos t} && (67)\\
=& \int_0^1 dq \int_0^1 dq' \frac{4qq'}{(x^2 + q^2 + q'^2)^2 - 4q^2 q'^2} && (68)\\
=& \int_0^1 du \int_0^1 du' \frac{1}{(x^2 + u + u')^2 - 4uu'} && (69)\\
=& \int_0^1 du \int_0^u du' \frac{2}{(x^2 + u + u')^2 - 4uu'} && (70)\\
=& \int_0^1 du \int_0^1 da \frac{2u}{(x^2 + u + au)^2 - 4au^2} && (71)\\
=& \int_0^1 du\, 2 \ln \frac{x^2 + |x|\sqrt{x^2 + 4}}{2x^2} && (72)\\
=& 2 \ln \left( \frac{1}{2} + \frac{\sqrt{x^2 + 4}}{2|x|} \right) - 1 + \frac{|x|}{2} \left( \sqrt{x^2 + 4} - |x| \right) && (73)
\end{aligned}$$

which after transformation gives Eq. (20) of the letter.

---

[1] Here, Maple definitions of the elliptic integrals are used. For computations, we use the GSL, where

$$\mathcal{E}_F^{\text{Maple}}(a, b) = \mathcal{E}_F^{\text{GSL}}(\arcsin(a), b) \tag{74}$$

$$\mathcal{E}_\pi^{\text{Maple}}(a, 1, b) = \mathcal{E}_\pi^{\text{GSL}}(\arcsin(a), b, -1) \tag{75}$$

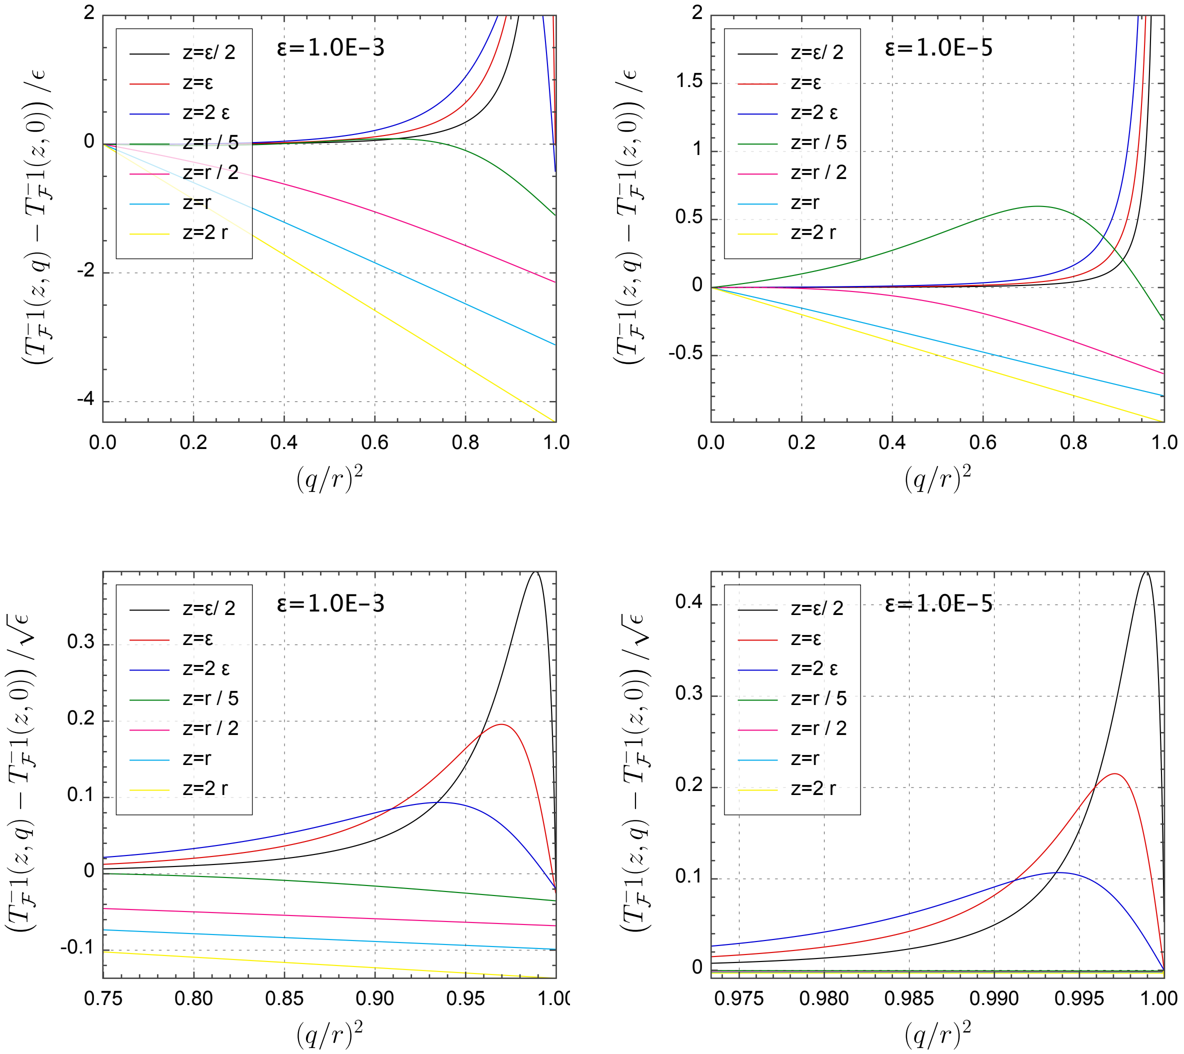


FIG. 2: Variations of $T_{\mathcal{F}}^{-}1(z,q)$ with respect to $q^2$ at various values of $z$. Left column stands for $\epsilon = 10^{-3}$ and right column for $\epsilon = 10^{-5}$. Top: $q$ varies between 0 and $r$. We see that for $r \gg \epsilon$, $T_{\mathcal{F}}^{-}1(z,q) - T_{\mathcal{F}}^{-}1(z,0)$ is quadratic in $q$. Moreover, these variations decrease faster than $\epsilon$. Bottom: Enlargement of the top-figures around $q = r$. $q$ varies between $r - 6\epsilon$ and $r$. We see that the maximum of the variations scales as $\sqrt{\epsilon}$
