# Supplementary material for: Upper bounds of spin-density wave energies in the homogeneous electron gas
Source: arXiv:1507.06884 source file (2015-07-24)
Supplement: Supplementary file 2 [file supp-SDW.pdf]

# Upper bounds of the Hartree-Fock energy in the homogeneous electron gas

F. Delyon,[1,2] B. Bernu,[2] L. Baguet,[2] and M. Holzmann[2,3]
[1]CPHT, UMR 7644 of CNRS, École Polytechnique, F-91128 Palaiseau Cedex, France
[2]LPTMC, UMR 7600 of CNRS, UPMC, Paris-Sorbonne, F-75252 Paris Cedex 05, France
[3]LPMMC, UMR 5493 of CNRS, Université J. Fourier, BP 166, F-38042 Grenoble Cedex, France

In this supplemental material, we provide technical details for the derivation of Eq.(23) and (25) of the letter.

PACS numbers:

## THE SDW ENERGY

The SDW energy is the energy variation when plane waves $|\mathbf{k},\uparrow\rangle$ are replaced by $a_{\mathbf{k}}\,|\mathbf{k},\uparrow\rangle + b_{\mathbf{k}}\,|\mathbf{k}+\mathbf{Q_k},\downarrow\rangle$ waves for $\mathbf{k}$ in the truncated Fermi sphere. Eq.18 of the main article provides this energy variation in the limit where the modulation depends only on the distance $x$ to the border of the truncated sphere:

$$\Delta E^{\mathcal{F}}_{\mathrm{SDW}} = \frac{4\pi a_V}{r_s} r^4\, \delta E^{\mathcal{F}}_{\mathrm{SDW}} \tag{1}$$

$$\delta E^{\mathcal{F}}_{\mathrm{SDW}} = 2\pi(\gamma x - 2x\ln(x), b^2) - (T^- b^2, b^2) - (T^+ ab, ab) \tag{2}$$

where the scalar product is now $(f,g) = \int_0^{1/r} dx\, f(x)g(x)$ and

$$b(x)^2 + a(x)^2 = 1 \tag{3}$$

$$0 \le b(x) \le 1/\sqrt{2} \tag{4}$$

and

$$(T^{\pm} f)(x) = \int_0^{1/r} dx' T^{\pm}(x,x') f(x') \tag{5}$$

$$T^{\pm}(x,x') = \pi\left(G(x-x') \pm G(x+x')\right) \tag{6}$$

where:

$$G(x) = G(|x|) = 2\ln\left(1+\frac{2}{|x|u}\right) - \frac{4}{u^2},\ u = |x| + \sqrt{x^2+4} \tag{7}$$

$\gamma$ is the large parameter of the problem ($\gamma$ is defined after Eq.4 of the letter, see Table I) and such that $\gamma > 2\ln(1/r)$

| parameter | definition |
|---|---|
| $a_V$ | $3/(32\pi^3)\,(9\pi/4)^{1/3}$ |
| $a_K/a_V$ | $2\pi^2\,(9\pi/4)^{1/3} \approx 37.9$ |
| $\alpha$ | $2(h-1/2)^2 + 1/6$ |
| $\gamma$ | $\ln(2/\epsilon) + a_K/(a_V \pi r_s)$ |

TABLE I: Constants and parameters defined in the letter. $h$ and $\epsilon$ are defined in Fig.1 and $r_s$ is the usual dimensionless parameter for the density.

ensuring that the first term in Eq.2 is positive. From the variations of Eq.2, the optimal $b$ satisfies:

$$\pi(\gamma x - 2x\ln(x)) - T^- b^2 - \frac{a^2-b^2}{2ab} T^+ ab = 0 \tag{8}$$

Setting $\xi = ab$, Eq.8 rewrites $\xi = J(\xi)$ where:

$$J(\xi) = \frac{1}{2}\frac{T^+\xi}{\sqrt{x^2\left(\pi(\gamma - 2\ln(x)) - T^- b^2\right)^2 + (T^+\xi)^2}}. \tag{9}$$

Afterwards, it will be checked that $-2\ln(x) - T^- b^2$ can be neglected at large $\gamma$. In the following, we just replace it with a constant, that is we replace $\gamma$ with $\gamma'$ and we expect that the solution of the simplified problem should provide a suitable upper bound for the energy. Thus here we consider the simpler problem of finding the fixed point of the operator $J_0$:

$$J_0(\xi) = \frac{1}{2}\frac{T^+\xi}{\sqrt{(\pi x\gamma')^2 + (T^+\xi)^2}}. \tag{10}$$

$\gamma'$ is now the large parameter of the problem. Now $\xi(x)$ can be considered as a positive function defined on $\mathbb{R}^+$ and accordingly $T^+$ must be defined by an integration over $\mathbb{R}^+$. As $J$, $J_0$ is monotonous i.e. if $f > g$, then $J_0(f) > J_0(g)$ and a fixed point is obtained as the limit of the sequence $\xi_n = J_0(\xi_{n-1})$, starting with $\xi_0 = 1/2$.

As $(T^+\xi)' = T^-(\xi')$, and $T^-$ is positivity preserving, if $\xi' \le 0$ then $(T^+\xi)' \le 0$. Then by Eq.10, $J(\xi)'$ is negative. Starting with $\xi_0 = 1/2$, we have $\xi_0' \le 0$ and by induction $\xi_n' \le 0$ and $T^+\xi_n' \le 0$. Thus setting $\eta = \lim \xi_n$, $\eta$ and $T^+\eta$ are decreasing functions.

Since $(T^+\xi)'(0) = 0$, for small $x$, the fixed point of $J_0$ behaves like:

$$\eta(x) \approx \eta_0(x) = \frac{1}{2}\frac{1}{\sqrt{(x/x_0)^2+1}} \tag{11}$$

$$x_0 = \frac{(T^+\eta)(0)}{\pi\gamma'} \tag{12}$$

And since $(T^+\eta)' \le 0$, we have:

$$\eta_0(x) \ge \eta(x) \ge \eta_0(x)\frac{T^+\eta(x)}{T^+\eta(0)}. \tag{13}$$

Indeed, by Eq.10 $J_0$ is an increasing function of $T^+\xi$ and $T^+\eta \geq T^+\eta(0)$. This gives the first inequality, the second is obtained replacing $T^+\eta$ by $T^+\eta(0)$ in the denominator of Eq.10.

As we shall see later $x_0$ is a very small parameter of order $\exp\left(-c\sqrt{\gamma'}\right)$. $G$ is positive and integrable, and $\eta \leq 1/2$, therefore $T^+\eta$ is integrable and, according to Eq.10, $\eta$ as well.

For non-zero finite $x$ ( $x \approx 1$), since $\eta_0$ is narrowed near zero and $G(x)$ is continuous, we have:

$$T^+\eta(x) \approx 2\pi G(x) \int_0^\infty \eta(x')dx' \tag{14}$$

and

$$\eta(x) \approx \frac{2G(x)}{\gamma' x_0}\eta_0(x) \int_0^\infty \eta(x')dx' \tag{15}$$

Unfortunately, this equation is not very useful because the behavior of $\eta$ mainly depends on what happens at small $x$.

Let us now look for the solution for $x < 1$. We first assume that the denominator of Eq.10 is in fact equivalent to $\sqrt{(\pi x\gamma')^2 + (T^+\eta(0))^2}$ for large $\gamma'$. In the following, we look for a solution of:

$$\eta(x) = \frac{1}{2}\frac{T^+\eta(x)}{\sqrt{(\pi x\gamma')^2 + (T^+\eta(0))^2}} = \eta_0\frac{T^+\eta(x)}{T^+\eta(0)}. \tag{16}$$

Setting

$$\eta = \eta_0 H \tag{17}$$

Eq.16 rewrites:

$$H = \frac{T^+ H\eta_0}{T^+\eta(0)}. \tag{18}$$

The second assumption is that the tail of $\eta$ is not relevant and thus we look for a solution of Eq.18 in a neighborhood of zero so that $G(x)$ may be approximated by $-\ln(x^2) - 1$ in the definition of $T^+$. Thus setting $x = x_0 \sinh\phi$ we look for a solution $H(\phi)$ for $\phi \in [0, \phi_0]$, and $H(\phi_0) \approx 0$. Eq.18 rewrites:

$$\gamma' H(\phi) = \int_0^{\phi_0} F(\phi,\phi')H(\phi')d\phi' \tag{19}$$

$$F(\phi,\phi') \approx -\ln(|\sinh(\phi) - \sinh(\phi')|) - \ln(|\sinh(\phi) + \sinh(\phi')|) - 2\ln x_0 - 1 \tag{20}$$

$$H(0) = 1,\ H(\phi_0) = 0 \tag{21}$$

The range for $\phi$ and $\phi'$ is large (say $(0, -\ln x_0)$), so that

$$\ln(|\sinh(\phi) \pm \sinh(\phi')|) \approx \max(\phi,\phi') - \ln 2 \tag{22}$$

except on the finite ranges $\phi' \approx \phi$ and $\phi' \approx \phi_0$. Thus:

$$F(\phi,\phi') \approx F_0(\phi,\phi') = 2(\phi_M - \max(\phi,\phi')) \tag{23}$$

$$\phi_M = -\ln x_0 + \ln 2 - \frac{1}{2} \tag{24}$$

as one can see on Fig.1. The peak occurring for $\phi \approx \phi'$ is roughly independent of $\phi$ and its total weight is $\frac{\pi^2}{6}$. Thus the weight of the peak is negligible with respect to $\gamma'$ at the left hand side of Eq.19. In the same way, near $\phi_0$, $\int |F - F_0|$ is finite and independent of $\gamma$.

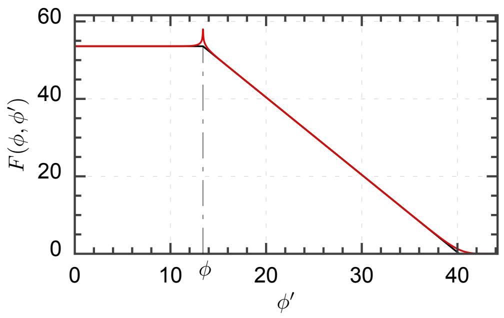


FIG. 1: $F(\phi,\phi')$ for $\ln x_0 = -40$. The red curve stands for the numerical computation of the exact kernel (from Eq.6). The black curve stand for Eq.23.

Now Eq.19 (with $F_0$) yields:

$$\gamma'\frac{dH(\phi)}{d\phi} = -2\int_0^\phi H(\phi')d\phi' \tag{25}$$

$$H(0) = 1,\ H(\phi_0) = 0 \tag{26}$$

That is:

$$H(\phi) = \cos\left(\sqrt{\frac{2}{\gamma'}}\phi\right) \tag{27}$$

$$\phi_0 = \frac{\pi}{2\sqrt{2}}\sqrt{\gamma'} \tag{28}$$

Finally, $x_0$ is given by Eq.12 i.e.:

$$\gamma' = \frac{T^+\eta(0)}{\pi x_0} \tag{29}$$

$$= \int_0^{\phi_0} F(0,\phi)H(\phi)d\phi \tag{30}$$

$$= \int_0^{\phi_0} 2(\phi_M - \phi)H(\phi)d\phi \tag{31}$$

$$= 2(\phi_M - \phi_0)\sqrt{\frac{\gamma'}{2}} + \gamma' \tag{32}$$

Thus $\phi_M = \phi_0$ and:

$$x_0 = 2\exp\left(-\frac{\pi}{2\sqrt{2}}\sqrt{\gamma'} - \frac{1}{2}\right) \tag{33}$$

and $F(\phi,\phi_0) = 0$.

Therefore the solution of Eq.16 is:

$$\eta(x) = \frac{1}{2\sqrt{\frac{x^2}{x_0^2} + 1}}\cos\left(\sqrt{\frac{2}{\gamma'}}\operatorname{arcsinh}\left(\frac{x}{x_0}\right)\right). \tag{34}$$

This solution satisfies the two above assumptions. Indeed the first assumption is equivalent to

$$\frac{x^2}{x_0^2}+1=\cosh(\phi)^2 \gg 1-H^2(\phi)=\sin^2\left(\sqrt{\frac{2}{\gamma'}}\phi\right) \quad (35)$$

which is in force for large $\gamma'$.

Let us now check the second assumption. Let $H_e(\phi)$ be the exact solution of Eq.16. Then $H_e$ satisfies:

$$\begin{aligned}\gamma' H_e(\phi) &= \int_0^{\phi_0} F(\phi,\phi')H_e(\phi')d\phi' + \int_{\phi_0}^{\infty} F(\phi,\phi')H_e(\phi')d\phi' \\ &\leq \int_0^{\phi_0} F(\phi,\phi')H_e(\phi')d\phi' + H_e(\phi)\int_{\phi_0}^{\infty} F(\phi,\phi')d\phi'\end{aligned} \quad (36)$$

with

$$\int_{\phi_M}^{\infty} F(\phi,\phi')d\phi' \leq 2\int_{1/\sqrt{e}}^{\infty} G(x-x')\eta_0(x')\frac{dx'}{x_0} \quad (37)$$

$$\leq \frac{2\eta_0(1/\sqrt{e})}{x_0}\int_0^{\infty} G(x-x')dx' \quad (38)$$

$$\leq \frac{16\sqrt{e}}{3} \quad (39)$$

Therefore

$$\int_{\phi_M}^{\infty} F(\phi,\phi')H_e(\phi')d\phi' \leq H_e(\phi)\frac{16\sqrt{e}}{3} \quad (40)$$

$$\ll \gamma' H_e(\phi) \quad (41)$$

and the tail of the exact solution $H_e$ is actually negligible as we can check on Fig.2.

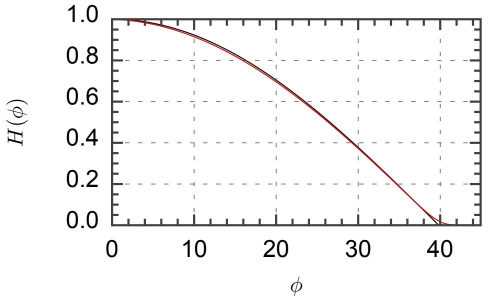


FIG. 2: $H(\phi)$ for $\ln x_0 = -40$. The red curve stands for numerical results with the exact kernel (from Eq.6). The black curve stand for Eq.34.

We can now compute by direct integration each term of $\delta E^{\mathcal{F}}_{\rm SDW}$ as in Appendix A:

$$\frac{\delta E^{\mathcal{F}}_{\rm SDW}(\eta)}{\pi x_0^2} = \frac{\pi^2-4}{32}\gamma' + \frac{\pi}{8\sqrt{2}}(\gamma-\gamma')\sqrt{\gamma'} + O\left(\sqrt{\gamma'}\right) \quad (42)$$

The minimum of $\delta E^{\mathcal{F}}_{\rm SDW}$ with respect to $\gamma'$ is for $2\pi\sqrt{2}(\gamma'-\gamma)=\sqrt{\gamma}(\pi^2+4)$:

$$\delta E^{\mathcal{F}}_{\rm SDW} \approx -\frac{\pi}{8}C\,\gamma e^{-\frac{\pi}{\sqrt{2}}\sqrt{\gamma}} \quad (43)$$

with $C=8e^{-3/2-\pi^2/8}$.

$$\Delta E^{\mathcal{F}}_{\rm SDW} \lesssim -\frac{2\pi^2 a_V}{r_s}C\epsilon^2\gamma\exp\left(-\frac{\pi}{\sqrt{2}}\sqrt{\gamma}\right). \quad (44)$$

## THE TOTAL ENERGY

Now we have to take into account the variation $\Delta E^{\mathcal{F}}_{\rm FG}$ in order to find the value of $\epsilon$ leading to the lowest energy.

We recall that $\Delta E^{\mathcal{F}}_{\rm FG}$ which is the Fermi energy difference of the truncated sphere and of the regular sphere is given by:

$$\Delta E^{\mathcal{F}}_{\rm FG} = \frac{2\pi^2 a_V}{r_s}\epsilon^3\gamma\alpha \quad (45)$$

Thus the energy gain of the SDW becomes:

$$\Delta E = \Delta E^{\mathcal{F}}_{\rm SDW} + \Delta E^{\mathcal{F}}_{\rm FG} \quad (46)$$

$$= \frac{2\pi^2 a_V}{r_s}\delta E \quad (47)$$

$$\delta E = \epsilon^3\gamma\alpha - C\epsilon^2\gamma\exp\left(-\frac{\pi}{\sqrt{2}}\sqrt{\gamma}\right) \quad (48)$$

where $\gamma$ depends on $\epsilon$ (see TableI).

The behavior of $\delta E$ is asymptotically dominated by the powers of $\epsilon$, thus the minimum with respect to $\epsilon$ occurs for:

$$3\times\epsilon^3\gamma\alpha - 2C\epsilon^2\gamma\exp\left(-\frac{\pi}{\sqrt{2}}\sqrt{\gamma}\right) \approx 0 \quad (49)$$

that is:

$$\epsilon \approx \frac{2C}{3\alpha}e^{-\frac{\pi^2}{4}}\exp\left(-\frac{\pi}{\sqrt{2}}\sqrt{\gamma_0}\right) \quad (50)$$

$$\approx \frac{0.0294e^{-7.714/\sqrt{r_s}}}{\alpha} \quad (51)$$

where $\gamma_0 = \frac{a_K}{a_V\pi r_s}$ depends only on $r_s$.

Finally:

$$\Delta E \approx -\frac{2\pi^2 a_V}{r_s}\frac{\gamma_0\alpha}{2}\epsilon^3 \quad (52)$$

$$= -0.69\,\alpha\frac{\epsilon^3}{r_s^2} \quad (53)$$

## APPENDIX A

In this appendix, we evaluate each term of the SDW energy with $\eta=\eta_0 H$ and $T^+\eta=\pi\gamma' x_0 H$ and $H$ is given by Eq.27.

The main difficulty is that some terms contain the function $b^2$. But $b^2 = \eta^2 + b^4$ and $b^4$ rewrites:

$$b^4 = \frac{4\eta^4}{(1+\sqrt{1-4\eta^2})^2} \le 4\eta^4 \tag{54}$$

thus $b^4$ rapidly decreases and leads to simple integrations at the leading order.

$$\begin{aligned}\delta E^{\mathcal{F}}_{\rm SDW} &= 2\pi(\gamma x - 2x\ln(x), b^2) - (T^- b^2, b^2) - (T^+\eta, \eta)\\ &= 2\pi\gamma'(x,\eta^2) - (T^+\eta,\eta) + 2\pi(\gamma-\gamma')(x,\eta^2)\\ &+ 2\pi\gamma(x,b^4) - 4\pi(x\ln\frac{x}{x_0}, b^2) - 4\pi\ln(x_0)(x,\, b^2)\\ &- (T^- b^2, b^2)\end{aligned} \tag{55}$$

1. **Evaluation of** $2\pi\gamma'(x,\eta^2) - (T^+\eta,\eta)$

   Here we set that $T^+\eta = T^+\eta(0)H$, i.e. we assume that $H$ is the solution of Eq.18.

$$2\pi\gamma'(x,\eta^2) - (T^+\eta,\eta) = \frac{\pi}{2}\gamma' x_0^2 \int H^2(\phi)(\tanh(\phi)-1)d\phi \tag{56}$$

$$= -\frac{\pi}{2}\gamma' x_0^2\ln(2) \tag{57}$$

$$+\frac{\pi}{2}\gamma' x_0^2 \int (H^2(\phi)-1)(\tanh(\phi)-1)d\phi \tag{58}$$

$$= -\frac{\pi}{2}\gamma' x_0^2\ln(2) + x_0^2 O(1) \tag{59}$$

2. **Evaluation of** $(x,b^2) = (x,\eta^2) + (x,b^4)$

   - **Evaluation of** $(x,\eta^2)$

$$\begin{aligned}(x,\eta^2) &= \int_0^\infty dx\, x\,\eta^2(x)\\ &= \frac{x_0^2}{4}\int_0^{\phi_0} dt\, \tanh(t)\, H(t)^2\\ &\approx \frac{x_0^2}{4}\left(\int_0^{\phi_0} dt\, H(t)^2 + \int_0^\infty dt\,(\tanh(t)-1)\right)\\ &= \frac{x_0^2}{4}\left(\frac{\phi_0}{2} - \ln 2 + O(1/\gamma)\right)\end{aligned} \tag{60}$$

   - **Evaluation of** $(x,b^4)$

$$\begin{aligned}(x,b^4) &= \int_0^\infty dx\, x\, \frac{4\eta(x)^4}{\left(1+\sqrt{1-4\eta^2}\right)^2}\\ &= \frac{x_0^2}{4}\int_0^{\phi_0} dt\, \frac{\sinh(t)}{\cosh(t)^3}\frac{H(t)^4}{(1+\sqrt{1-H(t)^2/\cosh(t)^2})^2}\\ &= \frac{x_0^2}{4}\int_0^{\phi_0} dt\, \frac{\sinh(t)H(0)^4}{\cosh(t)e^{2t}} + x_0^2 O(1/\gamma)\\ &= \frac{x_0^2}{4}\left(\ln 2 - \frac{1}{2}\right) + x_0^2 O(1/\gamma)\end{aligned} \tag{61}$$

$$(x,b^2) = \frac{x_0^2}{4}\left(\frac{\phi_0}{2} - 1/2 + O(1/\gamma)\right) \tag{62}$$

3. **Evaluation of** $(x\ln(x/x_0), b^2)$

$$(x\ln(x), b^2) = (x\ln(x/x_0),\eta^2) + (x\ln(x/x_0), b^4)$$

   - **Evaluation of** $(x\ln(x/x_0),\eta^2)$

$$\begin{aligned}\frac{4}{x_0^2}(x\ln(x/x_0),\eta^2) &= \int_0^{\phi_0} dt\, \ln(\sinh(t))\tanh(t)H^2(t)\\ &= \int_0^{\phi_0} dt\,(t-\ln 2)\tanh(t)H^2(t) + O(1)\\ &= \int_0^{\phi_0} dt\,(t-\ln 2)H^2(t) + O(1)\\ &= -\ln 2\frac{\phi_0}{2} + \frac{\gamma'}{2}\left(\frac{\pi^2}{16}-\frac{1}{4}\right) + O(1)\end{aligned} \tag{63}$$

   - **Evaluation of** $(x\ln(x/x_0), b^4)$

$$\begin{aligned}(x\ln(x/x_0), b^4) &\le 4(x\ln(x/x_0),\eta^4)\\ &\le 4(x\ln(x/x_0),\eta_0^4) = x_0^2 O(1)\end{aligned} \tag{64}$$

4. **Evaluation of** $(T^- b^2, b^2)$

$$(T^- b^2, b^2) = x_0^2 \times O(1) \tag{65}$$

Finally we have:

$$\begin{aligned}\frac{\delta E^{\mathcal{F}}_{\rm SDW}}{\pi x_0^2} &= (\gamma-\gamma')\frac{1}{4}\left(\frac{\pi}{2}\sqrt{\frac{\gamma'}{2}} - 1\right)\\ &+ \gamma'\frac{\pi^2-4}{32} - \frac{\pi}{8}\sqrt{\frac{\gamma'}{2}} + O(1)\end{aligned}$$
